# Supplementary material for: Deep Learning based Vulnerability Detection: Are We There Yet?
Source: arXiv:2009.07235 source file (2020-09-03)
Supplement: Supplementary file 1 [file A_pretrain_appendics.tex]

\subsection{Performance of existing models in predicting real world vulnerabilities.}
\label{appnd:pretrain_results}

We start with a straightforward question: how do the models trained with  (semi-)synthetic dataset perform on detecting real-world vulnerabilities. Without much of a surprise, we found that they perform poorly.

We use the vulnerability prediction models from
three existing techniques: (a)~ VulDeePecker~\cite{li2018vuldeepecker}, (b)~SySeVR~\cite{li2018sysevr}, and (c)~Russell~\etal~\cite{russell2018automated} to predict for vulnerabilities in the two real-world datasets examples FFMPeg + Qemu~\cite{zhou2019devign} and \realdata.

Table~\ref{tab:rq1_real_world_prediction} shows the performance of existing techniques for detecting real world vulnerability. For comparison, we tabulate the baseline results reported in the respective papers in the rows labeled ``baseline''. For baselines, VulDeePecker and SySeVR use a combination of NVD and SARD datasets for training and testing; Russell~\etal use GitHub + Debian for training and testing. We observe the following:

\noindent \textbf{VulDeePecker}. VulDeePecker works by extracting so called ``code gadgets'' from API function calls. We follow the same code-gadget extraction technique from \devigndata and \realdata. We could extract code gadgets from only \textit{27.96\% of the available code} in \devigndata and from \textit{only 21.46\% of the available code} in \realdata. Vulnerabilities in the rest of the code in both the datasets cannot be discovered by VulDeePecker. This is problematic because it leaves a large number of the real-world code unusable. In terms of predictive performance on the usable code, we observe that VulDeePecker performs significantly worse on both the real-world datasets. In \realdata, VulDeePecker achieves an F1-score of \textit{only} $\mathit{12.08}\%$ and in \devigndata VulDeePecker achieves an F1-score $\mathit{14.33}\%$, while in the baseline case which used semi-synthetic data for testing, the F1-score of VulDeePecker was as high as $85.4\%$.

\noindent \textbf{SySeVR}.  SySeVR works by extracting so ``code gadgets'' from API function calls, Array Usage, Arithmetic Operations, and  Pointer Usage. Using their technique, we could extract code gadgets from \textit{84.08\% of the available code} in \devigndata and from \textit{only 66.42\% of the available code} in \realdata. While this is higher than VulDeePecker, vulnerabilities in the rest of the code in both the datasets cannot be can still not be discovered by SySeVR. In terms of predictive performance on the usable code from real-world data, we observed that SySeVR still  performed significantly worse on both \realdata and \devigndata datasets. In \realdata, SySeVR achieved an F1-score of \textit{only} $\mathit{10.27}\%$ and in \devigndata SySeVR achieved an F1-score $\mathit{16.85}\%$, this was significantly lower than the F1-score of $85.2\%$ that was reported on baseline case which used semi-synthetic data for testing.

\noindent \textbf{Russell~\etal} Unlike the previous two techniques, Russell~\etal does not use code gadgets. Instead, Russell~\etal. tokenize available code and create abstract representation of the tokens to build their models. Therefore, they are able to perform predictions on 100\% of the available real-world data from \devigndata and \realdata. Even so, when we use the DL models offered by Russell~\etal on the real-world data from \realdata and \devigndata, we observe a notable reduction in predictive performance of the model. In the case of \devigndata, DL model from Russell~\etal's method produced an F1-score of $46.77\%$ on \devigndata compared to the baseline of $56.6\%$. In \realdata, the F1-score was only $23.67\%$.

We conjecture that the possible reason why Russell~\etal performs better than both VulDeePecker and SySeVR is due to the quality of the code used by each of the models to train their DLVP models. Both VulDeePecker and SySeVR are trained on NVD and SARD data. While NVD consists of real world production code, it only accounts for 7.85\%, 10.21\% of the total the training data in VulDeePecker and SySeVR respectively. Rest of the training examples belong to SARD dataset which is mostly synthetic and academic data. In contrast, all the code used for Russell~\etal's model come from open source repositories and the Debian distribution.
