# Supplementary material for: Deep Learning based Vulnerability Detection: Are We There Yet?
Source: arXiv:2009.07235 source file (2020-09-03)
Supplement: Supplementary file 2 [file D_scott_knott_all_comparison.tex]

\subsection{Scott-Knott rankings.}
\label{appnd:skott-knott-all}
\Cref{tab:scott_verum}, and \Cref{tab:scott_devign} show the relative ranking in terms of F1-score of \realdata and \devigndata respectively resulted by different approaches along with different variations of \tool. To generate this ranklist, we  used Scott-Knott procedure as described in \Cref{subsec:real-world-evaluation}.

\begin{table}[!tpb]
    \centering
    \scriptsize
    \caption{Relative rankings of different approaches based on F1-score in \realdata.}
    \begin{tabular}{l@{~~~}l@{~~~}r@{~~~}r@{~~~}c}
        \hlineB{2}
        \textbf{Rank} & \textbf{Approach} & \textbf{Median} & \textbf{IQR} & \textbf{Range}\bigstrut\\
        \hlineB{2}
          1 &       \tool &    41.25  &  2.28 & \quart{73}{6}{77}{233} \bigstrut\\
        \hline
          2 &          \tool-SVM &    39.81  &  2.50 & \quart{69}{6}{73}{233} \bigstrut\\
           & \tool-No-GGNN &    38.97  &  2.00 & \quart{68}{5}{70}{233} \bigstrut\\
        \hline
          3 & \tool-MLP$^\dagger$ &    30.62  &  3.36 & \quart{44}{9}{48}{233} \bigstrut\\
           &       SySeVR~\cite{li2018sysevr} &    30.25  &  2.35 & \quart{45}{7}{47}{233} \bigstrut\\
           &         GGNN &    29.87  &  4.34 & \quart{42}{11}{46}{233} \bigstrut\\
        \hline
          4 &   \tool-RF &    25.28  &  2.31 & \quart{30}{6}{34}{233} \bigstrut\\
        \hline
          5 & \tool-wo-SMOTE &    22.22  &  8.94 & \quart{13}{24}{26}{233} \bigstrut\\
        \hline
          6 & VulDeePecker~\cite{li2018vuldeepecker} &    15.70  &  6.41 & \quart{0}{17}{8}{233} \bigstrut\\
           & Russell \etal~\cite{russell2018automated} &    15.24  &  2.74 & \quart{2}{7}{7}{233} \bigstrut\\
        \hlineB{2}
    \end{tabular}
    \label{tab:scott_verum}
\end{table}

\begin{table}[!tpb]
    \centering
    \scriptsize
    \caption{Relative rankings of different approaches based on F1-score in \devigndata.}
    \begin{tabular}{l@{~~~}l@{~~~}r@{~~~}r@{~~~}c}
    \hlineB{2}
    \textbf{Rank} & \textbf{Approach} & \textbf{Median} & \textbf{IQR} & \bigstrut\\
    \hlineB{2}
      1 &       \tool &    64.42  &  1.33 & \quart{76}{3}{78}{161} \bigstrut\\
    \hline
      2 & \tool-No-GGNN &    63.67  &  0.83 & \quart{75}{2}{76}{161} \bigstrut\\
    \hline
      3 & \tool-MLP$^\dagger$ &    62.49  &  0.86 & \quart{73}{2}{73}{161} \bigstrut\\
    \hline
      4 & \tool-wo-SMOTE &    61.33  &  1.60 & \quart{69}{3}{71}{161} \bigstrut\\
    \hline
      5 &          \tool-SVM &    60.46  &  0.87 & \quart{67}{2}{69}{161} \bigstrut\\
    \hline
      6 &         \tool-GGNN &    57.18  &  2.58 & \quart{58}{6}{61}{161} \bigstrut\\
    \hline
      7 &       SySeVR~\cite{li2018sysevr} &    56.03  &  3.20 & \quart{53}{7}{58}{161} \bigstrut\\
    \hline
      8 &           \tool-RF &    52.19  &  1.06 & \quart{48}{2}{49}{161} \bigstrut\\
    \hline
      9 & Russell et. al.~\cite{russell2018automated} &    45.62  &  1.33 & \quart{32}{4}{34}{161} \bigstrut\\
    \hline
     10 & VulDeePecker~\cite{li2018vuldeepecker} &    35.20  &  8.82 & \quart{0}{20}{9}{161} \bigstrut\\
    \hlineB{2}
    \end{tabular}
    \label{tab:scott_devign}
\end{table}

% \begin{figure}[!tpb]
%     \input{Tables/lemna_example_1_integer_overflow}
%     \vspace{5mm}
%     \input{Tables/lemna_example_2_memory_overflow}
%     \vspace{5mm}
%     \input{Tables/lemna_example_3_draper_G_D}
%     % \vspace{5mm}
%     \caption{\small \textbf{Code examples visualization with Lemna~\cite{guo2018lemna}. All of these code examples are predicted as vulnerable by respective models. \cref{fig:lemna_int_overflow} and \cref{fig:lemna_memory_overflow} are code slices from NVD+SARD dataset and SySeVR predicted those as vulnerable. \cref{fig:lemna_draper} is also predicted as vulnerable by Russel~\etal's CNN+RF~\cite{russell2018automated} model. \lone{Red} colored tokens contributed the most in respective predictions. \lfive{Green} colored tokens contributed the least.}}
%     \label{fig:lemna_examples}
% \end{figure}

\begin{figure}
\centering
\begin{subfigure}{0.95\linewidth}
\scriptsize
\tt
\begin{tabular}{|r p{0.89\linewidth}|}
\hline
1  & \ltwo{link\_layer\_show(\textbf{struct} ib\_port {*}p, } \\
2  & ~~~~~~~\lone{\textbf{struct} port\_attribute {*}unused, \textbf{char} * buf)\{}\\
3  & ~~~\lone{\textbf{switch} }\lthree{(rdma\_port\_get\_link\_layer(}\\
4  & ~~~~~~~~~~~~~~~\lthree{p->ibdev, p->port\_num))}\lfive{ \{}\\
5  & ~~~~~~\lfive{\textbf{case} }\lfour{IB\_LINK\_LAYER\_INFINIBAND:}\\
6  & ~~~~~~~~~\lfour{\textbf{return} \blue{sprintf(buf, "\%s$\backslash$n", "InfiniBand")};}\\
7  & ~~~~~~\lfive{\textbf{case} IB\_LINK\_LAYER\_ETHERNET:}\\
8  & ~~~~~~~~~\lfive{\textbf{return} \blue{sprintf(buf, "\%s$\backslash$n", "Ethernet")};}\\
9  & ~~~~~~\lfive{\textbf{default}:}\\
10 & ~~~~~~~~~\lfive{\textbf{return} \blue{sprintf(buf, "\%s$\backslash$n", "Unknown")};}\\
11 & ~~~\lfive{\}}\\
12 & \lfive{\}}\\
\hline
\end{tabular}
\caption{{\small Vulnerable code example in \draper \cite{russell2018automated} dataset correctly predicted by a token-based Russel~\etal's method.}}
\label{fig:lemna_draper}
\end{subfigure}
\vspace{5mm}
    
\begin{subfigure}{0.95\linewidth}
\scriptsize
\tt
\begin{tabular}{|r p{0.89\linewidth}|}
\hline
1 & \textbf{static int} mov\_read\_dvc1(\lfour{MOVContext *c},  \\
2 & ~~~~~~~~\lfour{AVIOContext *pb}, \lthree{MOVAtom atom}) \{ \\
3 & ~~~~\lone{AVStream *st};  \\
4 & ~~~~\lfour{\textbf{uint8\_t} profile\_level}; \\
5 & ~~~~\textbf{if} (\lthree{c->fc->nb\_streams < 1}) \\ 
6 & ~~~~~~~~\lfour{\textbf{return} 0}; \\
7 & ~~~~\ltwo{st = c->fc->streams[c->fc->nb\_streams-1]}; \\
8 & ~~~~\textbf{if} (\lfour{atom.size $>=$ (1$<<$28) || atom.size $<$ 7}) \\
9 & ~~~~~~~~\lfour{\textbf{return} AVERROR\_INVALIDDATA}; \\
10 & ~~~~\lfour{profile\_level = avio\_r8(pb)}; \\
11 & ~~~~\textbf{if} (\lfour{(profile\_level \& 0xf0) $!=$ 0xc0}) \\
12 & ~~~~~~~~\lthree{\textbf{return} 0}; \\
...   & ~~~~...\\
% 13 & ~~~~\lfour{av\_free(st->codec->extradata)}; \\
% 14 & ~~~~\lfour{st->codec->extradata = av\_mallocz(}\\
% 15 & ~~~~\lfour{atom.size - 7 + FF\_INPUT\_BUFFER\_PADDING\_SIZE)}; \\
% 16 & ~~~~\textbf{if} (\lfive{$!$st->codec->extradata}) \\
% 17 & ~~~~~~~~\lfive{\textbf{return} AVERROR(ENOMEM)}; \\
18 & ~~~~\lfour{st->codec->extradata\_size = atom.size - 7}; \\
19 & ~~~~\ltwo{avio\_seek(pb, 6, SEEK\_CUR)}; \\
20 & ~~~~\lfour{\blue{{avio\_read(}}}\\
21 & ~~~~~~~~\lfour{\blue{{pb, st->codec->extradata,}}}\\
22 & ~~~~~~~~~~~~\lfour{\blue{{st->codec->extradata\_size)}}};\\ 
23 & ~~~~\lfour{\textbf{return} 0}; \\
24 & \}\\ 
\hline
\end{tabular}
\caption{{\small Vulnerable example from \devigndata~\cite{zhou2019devign} dataset correctly predicted by graph-based \tool model. Other methods could not predict the vulnerability in this example.}}
\label{fig:lemna_ggnn}
\end{subfigure}
\vspace{5mm}

\caption{Contribution of different code component in correctly  classifying the corresponding method as vulnerable by different models. \lone{Red-shaded} code elements have highest contribution, while  \lfive{Green-shaded} elements have the least. 
\blue{Blue} colored code are the source of vulnerabilities.}
\label{fig:code_heatmap}
\end{figure}

\Hide
{
\begin{figure}
\scriptsize
\begin{lstlisting}
static int mov_read_dvc1(@\lfour{MOVContext *c}@, 
	@\lfour{AVIOContext *pb}@, @\lthree{MOVAtom atom}@) { 
    @\lone{AVStream *st}@; 
    @\lfour{uint8\_t profile\_level}@; 
    if (@\lthree{c->fc->nb\_streams < 1}@) 
        @\lfour{return 0}@; 
    @\ltwo{st = c->fc->streams[c->fc->nb\_streams-1]}@; 
    if (@\lfour{atom.size $>=$ (1$<<$28) || atom.size $<$ 7}@) 
        @\lfour{return AVERROR\_INVALIDDATA}@; 
    @\lfour{profile\_level = avio\_r8(pb)}@; 
    if (@\lfour{(profile\_level \& 0xf0) $!=$ 0xc0}@) 
        @\lthree{return 0}@; 
    @\lfour{av\_free(st->codec->extradata)}@; 
    @\lfour{st->codec->extradata = av\_mallocz(}@
        @\lfour{atom.size - 7 + FF\_INPUT\_BUFFER\_PADDING\_SIZE)}@; 
    if (@\lfive{$!$st->codec->extradata}@) 
        @\lfive{return AVERROR(ENOMEM)}@; 
    @\lfour{st->codec->extradata\_size = atom.size - 7}@; 
    @\ltwo{avio\_seek(pb, 6, SEEK\_CUR)}@; 
    @\lfour{\red{\textbf{avio\_read(}}}@
        @\lfour{\red{\textbf{pb, st->codec->extradata,}}}@
        @\lfour{\red{\textbf{st->codec->extradata\_size)}}}@; 
    @\lfour{return 0}@; 
} 
\end{lstlisting}
\caption{\textbf{\small Devign Example.}}
\label{fig:devign_example_ggnn}
\end{figure}
}
