# Supplementary material for: Deep Learning based Vulnerability Detection: Are We There Yet?
Source: arXiv:2009.07235 source file (2020-09-03)
Supplement: Supplementary file 3 [file pretrain-full-result.tex]

%! TEX root = ../RQ_Details/rq1.tex

\begin{table}[htpb]
%\footnotesize
\centering
\scriptsize
\caption{\small Performance of Existing approaches in predicting real world vulnerability. Column SC refers to the sub-category under SySeVR's approach -- API refers to API calls, Arr-U referes to Array Usage, Arith refers to Arighmatic operation, and Pointer refers to Pointer Usage. Column ``Scope'' denoted percentage of code in real world datasets that are in the scope of a particular approach. Acc, Pr, Rc, F1 referes to Accuracy, Precision, Recall and F1-score respectively. Performance on Baseline dataset are respective models' performance when trained and evaluated on their datasets. The Baseline scores are taken from respective papers.}
\begin{tabular}{l|l|l|r|rrrr}
\hlineB{2}
\textbf{Dataset} & \textbf{Technique} & \textbf{SC} & \textbf{Scope} &  \textbf{Acc} & \textbf{Pr} & \textbf{Rc}   & \textbf{F1}\bigstrut\\ 
\hlineB{2}
& VulDeePecker 
   & N/A            & 21.46 & 78.97 & 13.50 & 10.93 & 12.08\bigstrut\\
\cline{2-8}
 & & API       & 21.46 & 69.93 & 11.73 & 19.54 & 14.66\bigstrut\\
 & & Arr-U  & 29.32 & 80.63 & 19.71 &  6.48 &  9.75\bigstrut\\
 & & Arith     & 30.39 & 80.76 & 15.87 &  6.15 &  8.87\bigstrut\\
 & & Pointer        & 52.69 & 86.44 & 15.69 &  5.20 &  7.81\bigstrut\\
 \cline{3-8}
 & \multirow{-5}{*}{SySeVR} & All        
                    & 66.42 & 79.44 & 15.75 &  9.34 & 10.27\bigstrut\\
 \cline{2-8}
\multirow{-7}{*}{\realdata} & Russel~\etal     
          &  N/A    &\red{100}& 70.06 & 15.60 & 49.00 & 23.67\bigstrut\\
\hlineB{2}
 & VulDeePecker 
 & N/A              & 27.96 & 52.27 & 44.96 & 8.50 & 14.33\bigstrut\\
\cline{2-8}
 & & API       & 27.96 & 52.59 & 43.56 & 4.16  &  7.60\bigstrut\\
 & & Arr-U    & 43.38 & 52.86 & 42.28 & 9.03  & 15.22\bigstrut\\
 & & Arith     & 45.62 & 50.63 & 46.51 & 18.35 & 26.31\bigstrut\\
 & & Pointer        & 52.69 & 53.90 & 48.67 & 11.25 & 18.25\bigstrut\\
 \cline{3-8}
 & \multirow{-5}{*}{SySeVR} & All        
                    & 84.08 & 52.50 & 42.26 & 10.70 & 16.85\bigstrut\\
 \cline{2-8}
\multirow{-7}{*}{\devigndata} & Russel~\etal     
          &  N/A    & \red{100}   & 54.04 & 49.63 & 44.22 & 46.77\bigstrut\\
\hlineB{2}
 & VulDeePecker 
 & N/A              & - & N/R & 86.90 & N/R & 85.4\bigstrut\\
\cline{2-8}
 & & API       & - & 94.9 & 87.3 & N/R  &  88.8\bigstrut\\
 & & Arr-U    & - & 92.4 & 82.5 & N/R  & 85.3\bigstrut\\
 & & Arith     & - & 97.3 & 87.5 & N/R & 87.5\bigstrut\\
 & & Pointer        & - & 96.9 & 80.2 & N/R & 83.2\bigstrut\\
 \cline{3-8}
 & \multirow{-5}{*}{SySeVR} & All        
                    & - & 95.9 & 82.5 & N/R & 85.2\bigstrut\\
 \cline{2-8}
\multirow{-7}{*}{Baseline} & Russel~\etal     
          &  N/A    & -   & N/R & N/R & N/R & 56.6\bigstrut\\
\hlineB{2}

\end{tabular}
N/R = Not Reported by the respective paper..
\label{tab:rq1_real_world_prediction}
\end{table}
