# Supplementary material for: Deep Learning based Vulnerability Detection: Are We There Yet?
Source: arXiv:2009.07235 source file (2020-09-03)
Supplement: Supplementary file 5 [file C_SMOTE_pseudocode.tex]

\subsection{Pseudocode for SMOTE}
\label{append:smote_code}

% def SMOTE(k=2, m=50%, r=2): # defaults
% while Majority > m do
% delete any majority item # random
% while Minority < m do
% add something_like(any minority item)
% def something_like(X0):
% relevant = emptySet
% k1 = 0
% while(k1++ < 20 and size(found) < k) {
% all = k1 nearest neighbors
% relevant += items in "all" of X0 class}
% Z = any of found
% Y = interpolate (X0, Z)
% return Y
% def minkowski_distance(a,b,r):
% return (Σi abs (ai − bi )
% r )
% 1/r

\begin{algorithm}[!tpb]
    \SetAlgoLined
    \footnotesize
    \SetKwInOut{Input}{Input}
    \SetKwInOut{Output}{Output}
    \SetKwFunction{SMOTE}{SMOTE}
    \SetKwProg{Fn}{Function}{:}{}
    \Input{Training Dataset -- $\mathbb{D}_\text{train}$\\
           Number of Nearest Neighbors -- $k$, \\
           Expected Number of samples per class -- $m$
         }
    \Output{Sampled Dataset -- $\mathbb{D}_\text{sampled}$.}
    % \Fn{\Fframework{$\mathbb{D}_\text{train}, \alpha, \beta, \gamma, lr$}}{
    \Fn{\SMOTE{$\mathbb{D}_\text{train}$, $k$, $m$}}{
        $\mathbb{D}_\text{sampled} \leftarrow \mathbb{D}_\text{train}$\\
        \While{\# of Majority examples $> m$}{
            $x \leftarrow $ random majority class example from $\mathbb{D}_\text{sampled}$\\
            Remove $x$ from $\mathbb{D}_\text{sampled}$\\
        }
        \While{\# of Minority examples $< m$}{
            $x \leftarrow $ random minority class example from $\mathbb{D}_\text{sampled}$\\
            $neighbors \leftarrow k$ nearest minority neighbors of $x$\\
            \For{$n \in neighbors$}{
                $x_s \leftarrow interpolate(x, n)$\\
                Add $x_s$ to $\mathbb{D}_\text{sampled}$\\
            }
        }
        \Return $\mathbb{D}_\text{sampled}$\\
    }
    \caption{\textbf{\small Algprithm for SMOTE.}}
    \label{alg:smote}
\end{algorithm}
