# Supplementary material for: Deep Learning based Vulnerability Detection: Are We There Yet?
Source: arXiv:2009.07235 source file (2020-09-03)
Supplement: Supplementary file 6 [file E_data_collection_algorithm.tex]

\begin{algorithm}[!htpb]
\footnotesize
\SetAlgoLined
\SetKwInOut{Input}{Input}
\SetKwInOut{Output}{Output}
\Input{List of Issues with patches($I_t$) from Issue tracker.}
\Output{List of Vulnerable(${V}$) and non-vulnerable(${N}$) code.}
 ${V}$ = ${N}$ = $set()$\;
 $V_i$ = filter\_vulnerability\_issues($I_t$)\;
 \For{$issue \in V_i$}{
  $patch$ = $issue$$\rightarrow$$getPatch()$\;
  $diff$ = $patch$$\rightarrow$$getDiffs()$\;
  \For{$file \in diff$}{
    \For{function $f_k \in file$}{
        \eIf{$f_k$ is changed in $patch$}{
            $f_k^p$ = $f_k$ before the change\;
            $f_k^n$ = $f_k$ after the change\;
            Add $f_k^p$ to ${V}$\;
            Add $f_k^n$ to ${N}$\;
        }{
            Add $f_k$ to ${N}$\;
        }
    }
  }
 }
 \textbf{return} ${V}$, ${N}$;
 \caption{\textbf{\small Algorithm for collecting vulneralble and non-vulnerable functions from open source code repository and issue tracker.}}
 \label{alg:real_data_collection}
\end{algorithm}
