# Supplementary material for: Deep Learning based Vulnerability Detection: Are We There Yet?
Source: arXiv:2009.07235 source file (2020-09-03)
Supplement: Supplementary file 8 [file main.tex]

% \subsection{Feature space of Representation Learning}
% \input{tex/t-sne}

% The graph embedding at the end of pre-processing tend to exhibit a high degree of overlap in feature space. This effect is illustrated by the t-SNE plot~\cite{maaten2008visualizing} of the feature space in~\fig{t-sne-train-plots}(a). In this example, there is no clear distinctions between the vulnerable  (denoted by \red{$\mathbf{+}$}) and the non-vulnerable samples (denoted by {$\mathbf{\circ}$}). This lack of separation makes it particularly difficult to train an ML model to learn the distinction between the vulnerable and the non-vulnerable samples.  After training the representation learning model with triplet loss we observe the better separability of the vulnerable and non-vulnerable examples in~\Cref{fig:t-sne-train-plots}(b).

% \subsection{Pseudocode for different components in \tool}
% \label{appends:code}
% Write about data collection
% \begin{algorithm}[!htpb]
% \footnotesize
% \SetAlgoLined
% \SetKwInOut{Input}{Input}
% \SetKwInOut{Output}{Output}
% \Input{List of Issues with patches($I_t$) from Issue tracker.}
% \Output{List of Vulnerable(${V}$) and non-vulnerable(${N}$) code.}
%  ${V}$ = ${N}$ = $set()$\;
%  $V_i$ = filter\_vulnerability\_issues($I_t$)\;
%  \For{$issue \in V_i$}{
%   $patch$ = $issue$$\rightarrow$$getPatch()$\;
%   $diff$ = $patch$$\rightarrow$$getDiffs()$\;
%   \For{$file \in diff$}{
%     \For{function $f_k \in file$}{
%         \eIf{$f_k$ is changed in $patch$}{
%             $f_k^p$ = $f_k$ before the change\;
%             $f_k^n$ = $f_k$ after the change\;
%             Add $f_k^p$ to ${V}$\;
%             Add $f_k^n$ to ${N}$\;
%         }{
%             Add $f_k$ to ${N}$\;
%         }
%     }
%   }
%  }
%  \textbf{return} ${V}$, ${N}$;
%  \caption{\textbf{\small Algorithm for collecting vulneralble and non-vulnerable functions from open source code repository and issue tracker.}}
%  \label{alg:real_data_collection}
% \end{algorithm}
% Algorithm \ref{alg:real_data_collection} shows the pseudo-code for \tool's data collection strategy. Recall from~\Cref{sect:tool_data_collection_section3}, \tool identifies the functions that are changed in a vulnerability-fix patch (line 3-7). \tool then adds the the version of those function before the change to the vulnerable set (line 11), and version after the change is applied to the non-vulnerable set (line 12). \tool considers all the function that are not changes as non-vulnerable. 
% % \subsection{Pseudocode for SMOTE}
% % \label{appends:smote_code}


%  Write about different components
% \input{tex/pseudo}
% Algorithm~\ref{alg:overview_psuedocode} shows the full training procedure for \tool. This algorithm expects Training data -- a list of tuples, where each tuple contains a code ($C$) and corresponding vulnerability annotation ($l$). \tool uses Algorithm~\ref{alg:feature_extraction} to extract graph embedding (graph based feature vector that represent the full code). Irrespective of the balance ratio (ratio of vulnerable and non-vulnerable examples) in the training set, \tool invokes SMOTE (see Algorithm~\ref{alg:smote}) to create a balance between number of samples from different classes. Finally Algorithm~\ref{alg:loss_function} is used to calculate the triplet loss (see \Cref{eqn:full_loss}). 
% \begin{algorithm}[!tpb]
%     \SetAlgoLined
%     \footnotesize
%     \SetKwInOut{Input}{Input}
%     \SetKwInOut{Output}{Output}
%     \SetKwFunction{SMOTE}{SMOTE}
%     \SetKwProg{Fn}{Function}{:}{}
%     \Input{Training Dataset -- $\mathbb{D}_\text{train}$\\
%           Number of Nearest Neighbors -- $k$, \\
%           Expected Number of samples per class -- $m$
%          }
%     \Output{Sampled Dataset -- $\mathbb{D}_\text{sampled}$.}
%     % \Fn{\Fframework{$\mathbb{D}_\text{train}, \alpha, \beta, \gamma, lr$}}{
%     \Fn{\SMOTE{$\mathbb{D}_\text{train}$, $k$, $m$}}{
%         $\mathbb{D}_\text{sampled} \leftarrow \mathbb{D}_\text{train}$\\
%         \While{\# of Majority examples $> m$}{
%             $x \leftarrow $ random majority class example from $\mathbb{D}_\text{sampled}$\\
%             Remove $x$ from $\mathbb{D}_\text{sampled}$\\
%         }
%         \While{\# of Minority examples $< m$}{
%             $x \leftarrow $ random minority class example from $\mathbb{D}_\text{sampled}$\\
%             $neighbors \leftarrow k$ nearest minority neighbors of $x$\\
%             \For{$n \in neighbors$}{
%                 $x_s \leftarrow interpolate(x, n)$\\
%                 Add $x_s$ to $\mathbb{D}_\text{sampled}$\\
%             }
%         }
%         \Return $\mathbb{D}_\text{sampled}$\\
%     }
%     \caption{\textbf{\small Pseudocode for SMOTE.}}
%     \label{alg:smote}
% \end{algorithm}


% \subsection{Impelmentation detail}
% \label{appneds:hparam}
% We use Pytorch 1.4.0 with Cuda version 10.1 to implement our method. For GGNN, we use tensorflow 1.15. We ran our experiments on single Nvidia Geforce 1080Ti GPU, Intel(R) Xeon(R) 2.60GHz 16 CPU with 252 GB ram. Neither Devign's implementation, nor their hyperparameters ate not publicly availavle. We followed their paper and re-implemented to our best ability. Pre-trained Word2Vec model used for initialization plays a very important role in Devign's performance. For the GGNN (both for Devign and \tool), We use Pytorch 1.4.0 with Cuda version 10.1 to implement our method. For GGNN, we use tensorflow 1.15. We ran our experiments on single Nvidia Geforce 1080Ti GPU, Intel(R) Xeon(R) 2.60GHz 16 CPU with 252 GB ram. For the GGNN, maximum iteration number is set to be 500. For the representation learner maximum iteration is 100. We stop the training procedure if F1-score on validation set does not increase in for 50 consecutive training iteration for GGNN and 5 for Representation Learning.  maximum iteration number is set to be 500. For the representation learner maximum iteration is 100. We stop the training procedure if F1-score on validation set does not increase in for 50 consecutive training iteration for GGNN and 5 for Representation Learning. We use Pytorch 1.4.0 with Cuda version 10.1 to implement our method. For GGNN, we use tensorflow 1.15. We ran our experiments on single Nvidia Geforce 1080Ti GPU, Intel(R) Xeon(R) 2.60GHz 16 CPU with 252 GB ram. For the GGNN, maximum iteration number is set to be 500. For the representation learner maximum iteration is 100. We stop the training procedure if F1-score on validation set does not increase in for 50 consecutive training iteration for GGNN and 5 for Representation Learning. Hyper-parameters for different components in \tool are shown in~\Cref{tab:hparams}.

% \begin{table}[!tpb]
%     \scriptsize
%     \centering
%     \caption{\small Hyper-parameter settings of \tool.}
%     \begin{tabular}{l|l|r}
%         \hlineB{2}
%         \textbf{Model} & \textbf{Parameter} & \textbf{Value} \bigstrut\\
%         \hlineB{2}
%         \multirow{2}{*}{Word2Vec} & Window Size & 10 \bigstrut\\
%         \cline{2-3}
%         & Vector Size & 100 \bigstrut\\
%         \hlineB{2}
%         & Input Embedding Size &  169 \bigstrut\\
%         \cline{2-3}
%         & Hidden Size & 200 \bigstrut\\
%         \cline{2-3}
%         & Number of Graph layers & 8 \bigstrut\\
%         \cline{2-3}
%         & Graph Activation Function & tanh \bigstrut\\
%         \cline{2-3}
%         \multirow{-7}{*}{GGNN}& Learning Rate & 0.0001\bigstrut\\
%         \hlineB{2}
%         & Number of hidden layers & 3 \bigstrut\\
%         \cline{2-3}
%         &Hidden layers sizes & 256, 128, 256\bigstrut\\
%         \cline{2-3}
%         &Hidden layer activation functions & relu\bigstrut\\
%         \cline{2-3}
%         &Dropout Probability & 0.2\bigstrut\\
%         \cline{2-3}
%         & $\gamma$ & 0.5\bigstrut\\
%         \cline{2-3}
%         & $\alpha$ & 0.5\bigstrut\\
%         \cline{2-3}
%         &$\beta$ & 0.001\bigstrut\\
%         \cline{2-3}
%         & Optimizer & Adam\bigstrut\\
%         \cline{2-3}
%         \multirow{-10}{*}{Repr-model} & $lr$ & 0.001\bigstrut\\
%         \hlineB{2}
%     \end{tabular}
%     \\Repr-model = Representation Learning Model used in \tool.
%     \label{tab:hparams}
% \end{table}

% \subsection{Ablation on different components of \tool}
% \label{appends:ablation}


% \input{RQ_answers/Tables/rq3_balancing}
% \input{RQ_answers/Tables/rq4_models}

% \Cref{tab:comparison_wo_ggnn}, \Cref{tab:comparison_wo_smote} show the effect of GGNN, SMOTE respectively in \tool's performance.~\Cref{fig:model_abl} shows the choice of different classification model in \tool's pipeline.

% \subsection{Complete comparison of different ablation results}
% \label{appends:comparison}

% \begin{table}[!tpb]
%     \centering
%     \scriptsize
%     \caption{Relative rankings of different approaches based on F1-score in \realdata.}
%     \begin{tabular}{l@{~~~}l@{~~~}r@{~~~}r@{~~~}c}
%         \hlineB{2}
%         \textbf{Rank} & \textbf{Approach} & \textbf{Median} & \textbf{IQR} & \textbf{Range}\bigstrut\\
%         \hlineB{2}
%           1 &       \tool &    41.25  &  2.28 & \quart{73}{6}{77}{233} \bigstrut\\
%         \hline
%           2 &          \tool-SVM &    39.81  &  2.50 & \quart{69}{6}{73}{233} \bigstrut\\
%           & \tool-No-GGNN &    38.97  &  2.00 & \quart{68}{5}{70}{233} \bigstrut\\
%         \hline
%           3 & \tool-MLP$^\dagger$ &    30.62  &  3.36 & \quart{44}{9}{48}{233} \bigstrut\\
%           &       SySeVR~\cite{li2018sysevr} &    30.25  &  2.35 & \quart{45}{7}{47}{233} \bigstrut\\
%           &         Devign &    29.87  &  4.34 & \quart{42}{11}{46}{233} \bigstrut\\
%         \hline
%           4 &   \tool-RF &    25.28  &  2.31 & \quart{30}{6}{34}{233} \bigstrut\\
%         \hline
%           5 & \tool-wo-SMOTE &    22.22  &  8.94 & \quart{13}{24}{26}{233} \bigstrut\\
%         \hline
%           6 & VulDeePecker~\cite{li2018vuldeepecker} &    15.70  &  6.41 & \quart{0}{17}{8}{233} \bigstrut\\
%           & Russell \etal~\cite{russell2018automated} &    15.24  &  2.74 & \quart{2}{7}{7}{233} \bigstrut\\
%         \hlineB{2}
%     \end{tabular}
%     \label{tab:scott_verum}
% \end{table}

% \begin{table}[!tpb]
%     \centering
%     \scriptsize
%     \caption{Relative rankings of different approaches based on F1-score in \devigndata.}
%     \begin{tabular}{l@{~~~}l@{~~~}r@{~~~}r@{~~~}c}
%     \hlineB{2}
%     \textbf{Rank} & \textbf{Approach} & \textbf{Median} & \textbf{IQR} & \bigstrut\\
%     \hlineB{2}
%       1 &       \tool &    64.42  &  1.33 & \quart{76}{3}{78}{161} \bigstrut\\
%     \hline
%       2 & \tool-No-GGNN &    63.67  &  0.83 & \quart{75}{2}{76}{161} \bigstrut\\
%     \hline
%       3 & \tool-MLP$^\dagger$ &    62.49  &  0.86 & \quart{73}{2}{73}{161} \bigstrut\\
%     \hline
%       4 & \tool-wo-SMOTE &    61.33  &  1.60 & \quart{69}{3}{71}{161} \bigstrut\\
%     \hline
%       5 &          \tool-SVM &    60.46  &  0.87 & \quart{67}{2}{69}{161} \bigstrut\\
%     \hline
%       6 &         Devign &    57.18  &  2.58 & \quart{58}{6}{61}{161} \bigstrut\\
%     \hline
%       7 &       SySeVR~\cite{li2018sysevr} &    56.03  &  3.20 & \quart{53}{7}{58}{161} \bigstrut\\
%     \hline
%       8 &           \tool-RF &    52.19  &  1.06 & \quart{48}{2}{49}{161} \bigstrut\\
%     \hline
%       9 & Russell et. al.~\cite{russell2018automated} &    45.62  &  1.33 & \quart{32}{4}{34}{161} \bigstrut\\
%     \hline
%      10 & VulDeePecker~\cite{li2018vuldeepecker} &    35.20  &  8.82 & \quart{0}{20}{9}{161} \bigstrut\\
%     \hlineB{2}
%     \end{tabular}
%     \label{tab:scott_devign}
% \end{table}

% \Cref{tab:scott_verum}, and \Cref{tab:scott_devign} show the relative ranking in terms of F1-score of \realdata and \devigndata respectively resulted by different approaches along with different variations of \tool. To generate this ranklist, we  used Scott-Knott procedure as described in \Cref{subsec:real-world-evaluation}. If two methods shares same rank, that indicates, the difference between those methods are statistically insignificant. For instance, \tool-MLP$^{\dagger}$, SySeVR, Devign in \Cref{tab:scott_verum} have different median F1 scores, but their ranges are not statistically significantly different from each other. While doing statistical significance test, we used p-value 99\% and A12 effect-size $\ge$ 0.6. 
