# Supplementary material for: Deep Learning based Vulnerability Detection: Are We There Yet?
Source: arXiv:2009.07235 source file (2020-09-03)
Supplement: Supplementary file 9 [file previsous_resclone.tex]

\begin{table}[!tb]
    \centering
    \scriptsize
    \caption{\small Percentage of duplicate samples in datasets. Draper data provide specific train, dev, and test split of the dataset. 94.93\% examples are unique to dev and test set from the corresponding train set. We found 97.02\% unique examples when we combine all the examples together.}
    \begin{tabular}{c|c|c}
        \hlineB{2}
        \textbf{Dataset} &\textbf{Sub-Category / Used by} & \textbf{\% of duplicates samples}\bigstrut\\
        \hlineB{2}
         Juliet & - / Russel~\etal & 57.00 \bigstrut\\
         \hlineB{1}
         \multirow{6}{*}{NVD + SARD} & CWE119 / VulDeePecker &  62.79 \bigstrut\\
         & CWE399 / VulDeePecker & 74.81 \bigstrut\\
         & API-Call / SySeVR &  44.61 \bigstrut\\
         & Array-Usage / SySeVR &  57.49 \bigstrut\\
         & Arith-Expr / SySeVR &  43.51 \bigstrut\\
         & Pointer / SySeVR &  54.58 \bigstrut\\
         \hlineB{1}
         Draper & - / Russel~\etal & 6.07 / 2.99 \bigstrut\\
         \hlineB{2}
    \end{tabular}
    \label{tab:duplicate}
\end{table}
