# Supplementary material for: Deep Learning based Vulnerability Detection: Are We There Yet?
Source: arXiv:2009.07235 source file (2020-09-03)
Supplement: Supplementary file 10 [file retrain.tex]

\begin{table*}[!htpb]
    \centering
    \scriptsize
    \caption{\small Result of different approaches when trained on Real World Data.}
    \begin{tabular}{l|l|l|r|r|r|r|r}
        \hlineB{2}
        \multirow{2}{*}{\textbf{Dataset}} & \textbf{Approach} & \multirow{2}{*}{\textbf{Approach}} & \textbf{\% samples} & \textbf{Accuracy} & \textbf{Precision}  & \textbf{Recall} & \textbf{F1-score}\\
        & \textbf{Type} & & \textbf{in-scope} &\multicolumn{4}{c}{\textbf{average $\pm$ standard\_deviation}}\\
        \hlineB{2}
        \multirow{7}{*}{\realdata} & \multirow{3}{*}{Token based} & VulDeePecker & 21.46 & 81.49 $\pm$ 1.82 & 38.85 $\pm$ 3.41 & 54.26 $\pm$ 9.74 & 44.91 $\pm$ 4.43 \bigstrut\\
        \cline{3-8}
        && SySeVR & 66.42 & 87.22 $\pm$ 1.40 & 59.86 $\pm$ 4.64 & 69.46 $\pm$ 11.29 & 63.82 $\pm$ 5.91 \bigstrut\\
        \cline{3-8}
        && Russel~\etal & 100 & 91.39 $\pm$ 0.45 & 28.01 $\pm$ 1.45 & 15.59 $\pm$ 1.23 & 19.98 $\pm$ 1.06 \bigstrut\\
        \cline{2-8}
        &\multirow{3}{*}{Graph + ML} & SVM & 100 & 87.16 $\pm$ 2.70 & 14.31 $\pm$ 3.20 & 14.92 $\pm$ 8.98 & 12.93 $\pm$ 5.77 \bigstrut\\
        \cline{3-8}
       & & LR & 100 & 90.75 $\pm$ 0.16 & 22.76 $\pm$ 7.72 & 4.40 $\pm$ 1.81 & 7.07 $\pm$ 2.54 \bigstrut\\
        \cline{3-8}
        && KNN & 100 & 89.83 $\pm$ 0.53 & 29.15 $\pm$ 2.03 & 13.73 $\pm$ 3.27 & 18.43 $\pm$ 3.22 \bigstrut\\
        \cline{2-8}
       & Graph + DL& GGNN & 100 & 79.38 $\pm$ 1.58 & 23.94 $\pm$ 1.69 & 65.47 $\pm$ 4.74 & 35.00 $\pm$ 2.10 \bigstrut\\
       \hlineB{2}
        \multirow{7}{*}{\devigndata} & \multirow{3}{*}{Token based} & VulDeePecker & 
        27.96 & 57.94 $\pm$ 3.34 & 56.91 $\pm$ 3.71 & 55.86 $\pm$ 9.37 & 59.94 $\pm$ 4.86 \bigstrut\\
        \cline{3-8}
        && SySeVR & 84.08 & 67.91 $\pm$ 2.10 & 64.63 $\pm$ 1.13 & 78.46 $\pm$ 0.85 & 70.87 $\pm$ 0.70 \bigstrut\\
        \cline{3-8}
        && Russel~\etal & 100 & 57.42 $\pm$ 0.55 & 53.31 $\pm$ 2.22 & 38.93 $\pm$ 1.02 & 44.98 $\pm$ 1.11 \bigstrut\\
        \cline{2-8}
        &\multirow{3}{*}{Graph + ML} & SVM & 100 & 54.07 $\pm$ 1.39 & 47.44 $\pm$ 0.95 & 37.92 $\pm$ 9.51 & 41.47 $\pm$ 6.33 \bigstrut\\
        \cline{3-8}
       & & LR & 100 & 57.65 $\pm$ 0.52 & 55.12 $\pm$ 0.62 & 34.51 $\pm$ 2.17 & 42.40 $\pm$ 4.62 \bigstrut\\
        \cline{3-8}
        && KNN & 100 & 60.77 $\pm$ 0.31 & 56.03 $\pm$ 0.51 & 53.87 $\pm$ 0.82 & 54.93 $\pm$ 0.52 \bigstrut\\
        \cline{2-8}
       & Graph + DL& GGNN & 100 & 62.18 $\pm$ 2.43 & 56.27 $\pm$ 3.81 & 65.49 $\pm$ 4.17 & 60.40 $\pm$ 2.75 \bigstrut\\
        \hlineB{2}
    \end{tabular}
    \label{tab:all_method_comparison_real_world_datasets}
\end{table*}
